# Supplementary material for: A machine learning approach for efficient uncertainty quantification using multiscale methods
Source: arXiv:1711.04315 source file (2017-11-12)
Supplement: Supplementary file 1 [file appendix.tex]

\section{Appendix}
\subsection{Dropout}
\begin{figure}
  \centering
  \includegraphics[width=.7\textwidth]{fig/dropout}
  \caption{Illustration of dropout in action.}
  \label{fig:dropout}
\end{figure}

Dropout \cite{srivastava2014dropout} is a regularization technique developed specifically to
address the difficulties of \emph{averaging} in neural
networks. Because large networks are expensive to train, and
evaluating a large number of them would be slow, model averaging in
neural networks becomes limited to small models. Dropout essentially
attempts to approximate model averaging by randomly dropping out units
of the network during
training. Figure~\ref{fig:dropout}\footnote{Figure taken from
  \cite{srivastava2014dropout}} illustrates this process. By doing
this, the optimization procedure ``sees'' an exponential number of
similar but different models during training as a consequence of the
different networks that are obtained by randomly dropping out some
units. Another explanation of the effectiveness of dropout is that it
prevents the units from co-adaptation.

A \emph{dropout rate} is a number between $0$ and $1$ defining the
probability that a unit is dropped out. In practice, when a
\emph{dropout layer} of rate $r$ is imposed after a given layer of the
network, it means that each unit of such given layer has a probability
$r$ to be dropped out. The dropout paper suggests default values of
$10\%$ after the input layer and $20\%$ to $50\%$ after hidden layers,
although these guidelines resulted from numerical experiments in
computer vision.
